# Supplementary material for: Quantitative experimental observation of weak inertial-wave turbulence
Source: arXiv:2010.15563 ancillary file (2020-10-29)
Supplement: Supplementary file 1 [file Monsalve_PRL_SM.pdf]

# —Supplemental Material—
# Quantitative experimental observation of weak inertial-wave turbulence

Eduardo Monsalve,[1] Maxime Brunet,[1] Basile Gallet,[2] and Pierre-Philippe Cortet[1]
[1] *Université Paris-Saclay, CNRS, FAST, 91405, Orsay, France*
[2] *Université Paris-Saclay, CNRS, CEA, Service de Physique de l'État Condensé, 91191, Gif-sur-Yvette, France*

As described in Ref. [1], the standard calculations of Weak Turbulence Theory can be performed by considering a finite domain with periodic boundary conditions. One then introduces a weak-amplitude expansion, before considering ensemble averages under the random-phase approximation, followed by the infinite-domain and long-time limits. We detail here the precise conventions considered when discussing the asymptotic expansion in small Rossby number in a finite domain with periodic boundary conditions.

Following Smith & Waleffe [2], we decompose the velocity field onto the wavevectors of a triply periodic box, using a helical basis:

$$\mathbf{u} = \Sigma_{\mathbf{k}} \Sigma_{s=\pm 1} b_s(\mathbf{k},t) \mathbf{h}_s(\mathbf{k})\, e^{i[\mathbf{k}\cdot\mathbf{x} - \omega_s(\mathbf{k})t]}\,, \tag{1}$$

where the first sum is over all wavevectors $\mathbf{k}$. The helical basis vectors $\mathbf{h}_s(\mathbf{k})$ are defined as:

$$\mathbf{h}_s(\mathbf{k}) = \hat{\mathbf{k}} \times \frac{\mathbf{k}\times\hat{\mathbf{z}}}{|\mathbf{k}\times\hat{\mathbf{z}}|} + i\, s \frac{\mathbf{k}\times\hat{\mathbf{z}}}{|\mathbf{k}\times\hat{\mathbf{z}}|}\,, \tag{2}$$

where $\hat{\mathbf{z}}$ is the unit vector in the vertical direction, and $\hat{\mathbf{k}} = \mathbf{k}/|\mathbf{k}|$. The reality constraint for the velocity field imposes $b_s(\mathbf{k},t) = b_s^*(-\mathbf{k},t)$. The helical basis vectors correspond to the spatial structure of inertial-wave modes, the frequency $\omega_s(\mathbf{k})$ of the mode at wavenumber $\mathbf{k}$ with polarity $s$ being given by the dispersion relation:

$$\omega_s(\mathbf{k}) = 2\Omega\, s\, \frac{\mathbf{k}\cdot\hat{\mathbf{z}}}{k}\,, \tag{3}$$

where $k = |\mathbf{k}|$.

Inserting the decomposition (1) into the rotating Euler equation leads to:

$$\partial_t b_{s_\mathbf{k}} = \frac{1}{2} \sum C_{\mathbf{kpq}}^{s_\mathbf{k} s_\mathbf{p} s_\mathbf{q}} b_{s_\mathbf{p}}^* b_{s_\mathbf{q}}^* e^{i(\omega_{s_\mathbf{k}} + \omega_{s_\mathbf{p}} + \omega_{s_\mathbf{q}})t}\,. \tag{4}$$

This is the inviscid version of equation (5) in Smith & Waleffe [2]. The sum is over all wavenumbers $\mathbf{p}$ and $\mathbf{q}$ such that $\mathbf{k}+\mathbf{p}+\mathbf{q} = \mathbf{0}$, and over the polarities $s_\mathbf{p} = \pm 1$, $s_\mathbf{q} = \pm 1$. The triadic interaction coefficients are:

$$C_{\mathbf{kpq}}^{s_\mathbf{k} s_\mathbf{p} s_\mathbf{q}} = \frac{s_q q - s_p p}{2} \left[\mathbf{h}_{s_p}^*(\mathbf{p}) \times \mathbf{h}_{s_q}^*(\mathbf{q})\right] \cdot \mathbf{h}_{s_k}^*(\mathbf{k})\,. \tag{5}$$

We non-dimensionalize Eq. (4) using the timescale $\Omega^{-1}$ and a length scale $L$ (for instance, the typical wavelength associated with the forced wave beams):

$$\partial_{\tilde{t}} \tilde{b}_{s_{\tilde{\mathbf{k}}}} = \frac{1}{2} \sum C_{\tilde{\mathbf{k}}\tilde{\mathbf{p}}\tilde{\mathbf{q}}}^{s_\mathbf{k} s_\mathbf{p} s_\mathbf{q}} \tilde{b}_{s_{\tilde{\mathbf{p}}}}^* \tilde{b}_{s_{\tilde{\mathbf{q}}}}^* e^{i(\tilde{\omega}_{s_{\tilde{\mathbf{k}}}} + \tilde{\omega}_{s_{\tilde{\mathbf{p}}}} + \tilde{\omega}_{s_{\tilde{\mathbf{q}}}})\tilde{t}}\,, \tag{6}$$

where $\tilde{t} = \Omega t$, $\tilde{\mathbf{k}} = \mathbf{k}L$, $\tilde{b}_{s_{\tilde{\mathbf{k}}}} = b_{s_\mathbf{k}}/L\Omega$, and $\tilde{\omega}_{s_{\tilde{\mathbf{k}}}} = \omega_{s_\mathbf{k}}/\Omega$. We drop the tildes in the following to alleviate notations. For rapid global rotation, the Rossby number based on the root-mean-square velocity $U$ is small, $Ro = U/2L\Omega \ll 1$. We introduce a multiple timescale expansion:

$$b_{s_\mathbf{k}} = Ro\, b_{s_\mathbf{k}}^{(0)}(t, T_1, T_2, \dots) + Ro^2 b_{s_\mathbf{k}}^{(1)}(t, T_1, T_2, \dots) + Ro^3 b_{s_\mathbf{k}}^{(2)}(t, T_1, T_2, \dots) + \dots\,, \tag{7}$$

where the slow time variables are $T_1 = Ro\, t$, $T_2 = Ro^2\, t$ and so on. Inserting this expansion into Eq. (6) and collecting terms at order $\mathcal{O}(Ro)$ yields simply:

$$\partial_t b_{s_\mathbf{k}}^{(0)} = 0\,, \tag{8}$$

i.e., the wave amplitudes do not vary on the fast timescale.

To order $\mathcal{O}(Ro^2)$, Eq. (6) yields:

$$\partial_t b_{s_\mathbf{k}}^{(1)} + \partial_{T_1} b_{s_\mathbf{k}}^{(0)} = \frac{1}{2} \sum C_{\mathbf{kpq}}^{s_\mathbf{k} s_\mathbf{p} s_\mathbf{q}}\, b_{s_\mathbf{p}}^{*\,(0)}\, b_{s_\mathbf{q}}^{*\,(0)}\, e^{i(\omega_{s_\mathbf{k}} + \omega_{s_\mathbf{p}} + \omega_{s_\mathbf{q}})t}\,. \tag{9}$$

Averaging the right-hand side with respect to the fast variable $t$ gives zero, except for resonant triads: if $\omega_{s_\mathbf{k}} + \omega_{s_\mathbf{p}} + \omega_{s_\mathbf{q}} = 0$, then the fast-time average is non-zero. When this is the case, we obtain $\partial_{T_1} b^{(0)}_{s_\mathbf{k}} \neq 0$ when averaging (9): this evolution with time $T_1$ corresponds to the standard nonlinear interactions within resonant triads of waves. Upon subtracting the $t$-average of (9) from the full Eq. (9), we obtain:

$$\partial_t b^{(1)}_{s_\mathbf{k}} = \frac{1}{2} \sum_{\omega_{s_\mathbf{k}}+\omega_{s_\mathbf{p}}+\omega_{s_\mathbf{q}}\neq 0} C^{s_\mathbf{k} s_\mathbf{p} s_\mathbf{q}}_{\mathbf{kpq}} \, b^{*\,(0)}_{s_\mathbf{p}} \, b^{*\,(0)}_{s_\mathbf{q}} \, e^{i(\omega_{s_\mathbf{k}}+\omega_{s_\mathbf{p}}+\omega_{s_\mathbf{q}})t} \, . \tag{10}$$

The sum is still over all values of the wave vectors $\mathbf{p}$ and $\mathbf{q}$ such that $\mathbf{k}+\mathbf{p}+\mathbf{q}=0$, and over the polarities $s_\mathbf{p} = \pm 1$, $s_\mathbf{q} = \pm 1$, but omitting the resonant triads, that satisfy $\omega_{s_\mathbf{k}} + \omega_{s_\mathbf{p}} + \omega_{s_\mathbf{q}} = 0$. The solution to this equation is:

$$b^{(1)}_{s_\mathbf{k}} = -\frac{i}{2} \times \sum_{\omega_{s_\mathbf{k}}+\omega_{s_\mathbf{p}}+\omega_{s_\mathbf{q}}\neq 0} C^{s_\mathbf{k} s_\mathbf{p} s_\mathbf{q}}_{\mathbf{kpq}} \, \frac{b^{*\,(0)}_{s_\mathbf{p}} \, b^{*\,(0)}_{s_\mathbf{q}}}{\omega_{s_\mathbf{k}} + \omega_{s_\mathbf{p}} + \omega_{s_\mathbf{q}}} \, e^{i(\omega_{s_\mathbf{k}}+\omega_{s_\mathbf{p}}+\omega_{s_\mathbf{q}})t} \, . \tag{11}$$

[1] S. Nazarenko, *Wave Turbulence* (Springer, Berlin, 2011).
[2] L.M. Smith and F. Waleffe, Phys. Fluids **11**, 1608 (1999).
